# Supplementary material for: A single-chain nanoparticle-based mean-field theory for associative polymers
Source: arXiv:2512.16405 source file (2026-06-15)

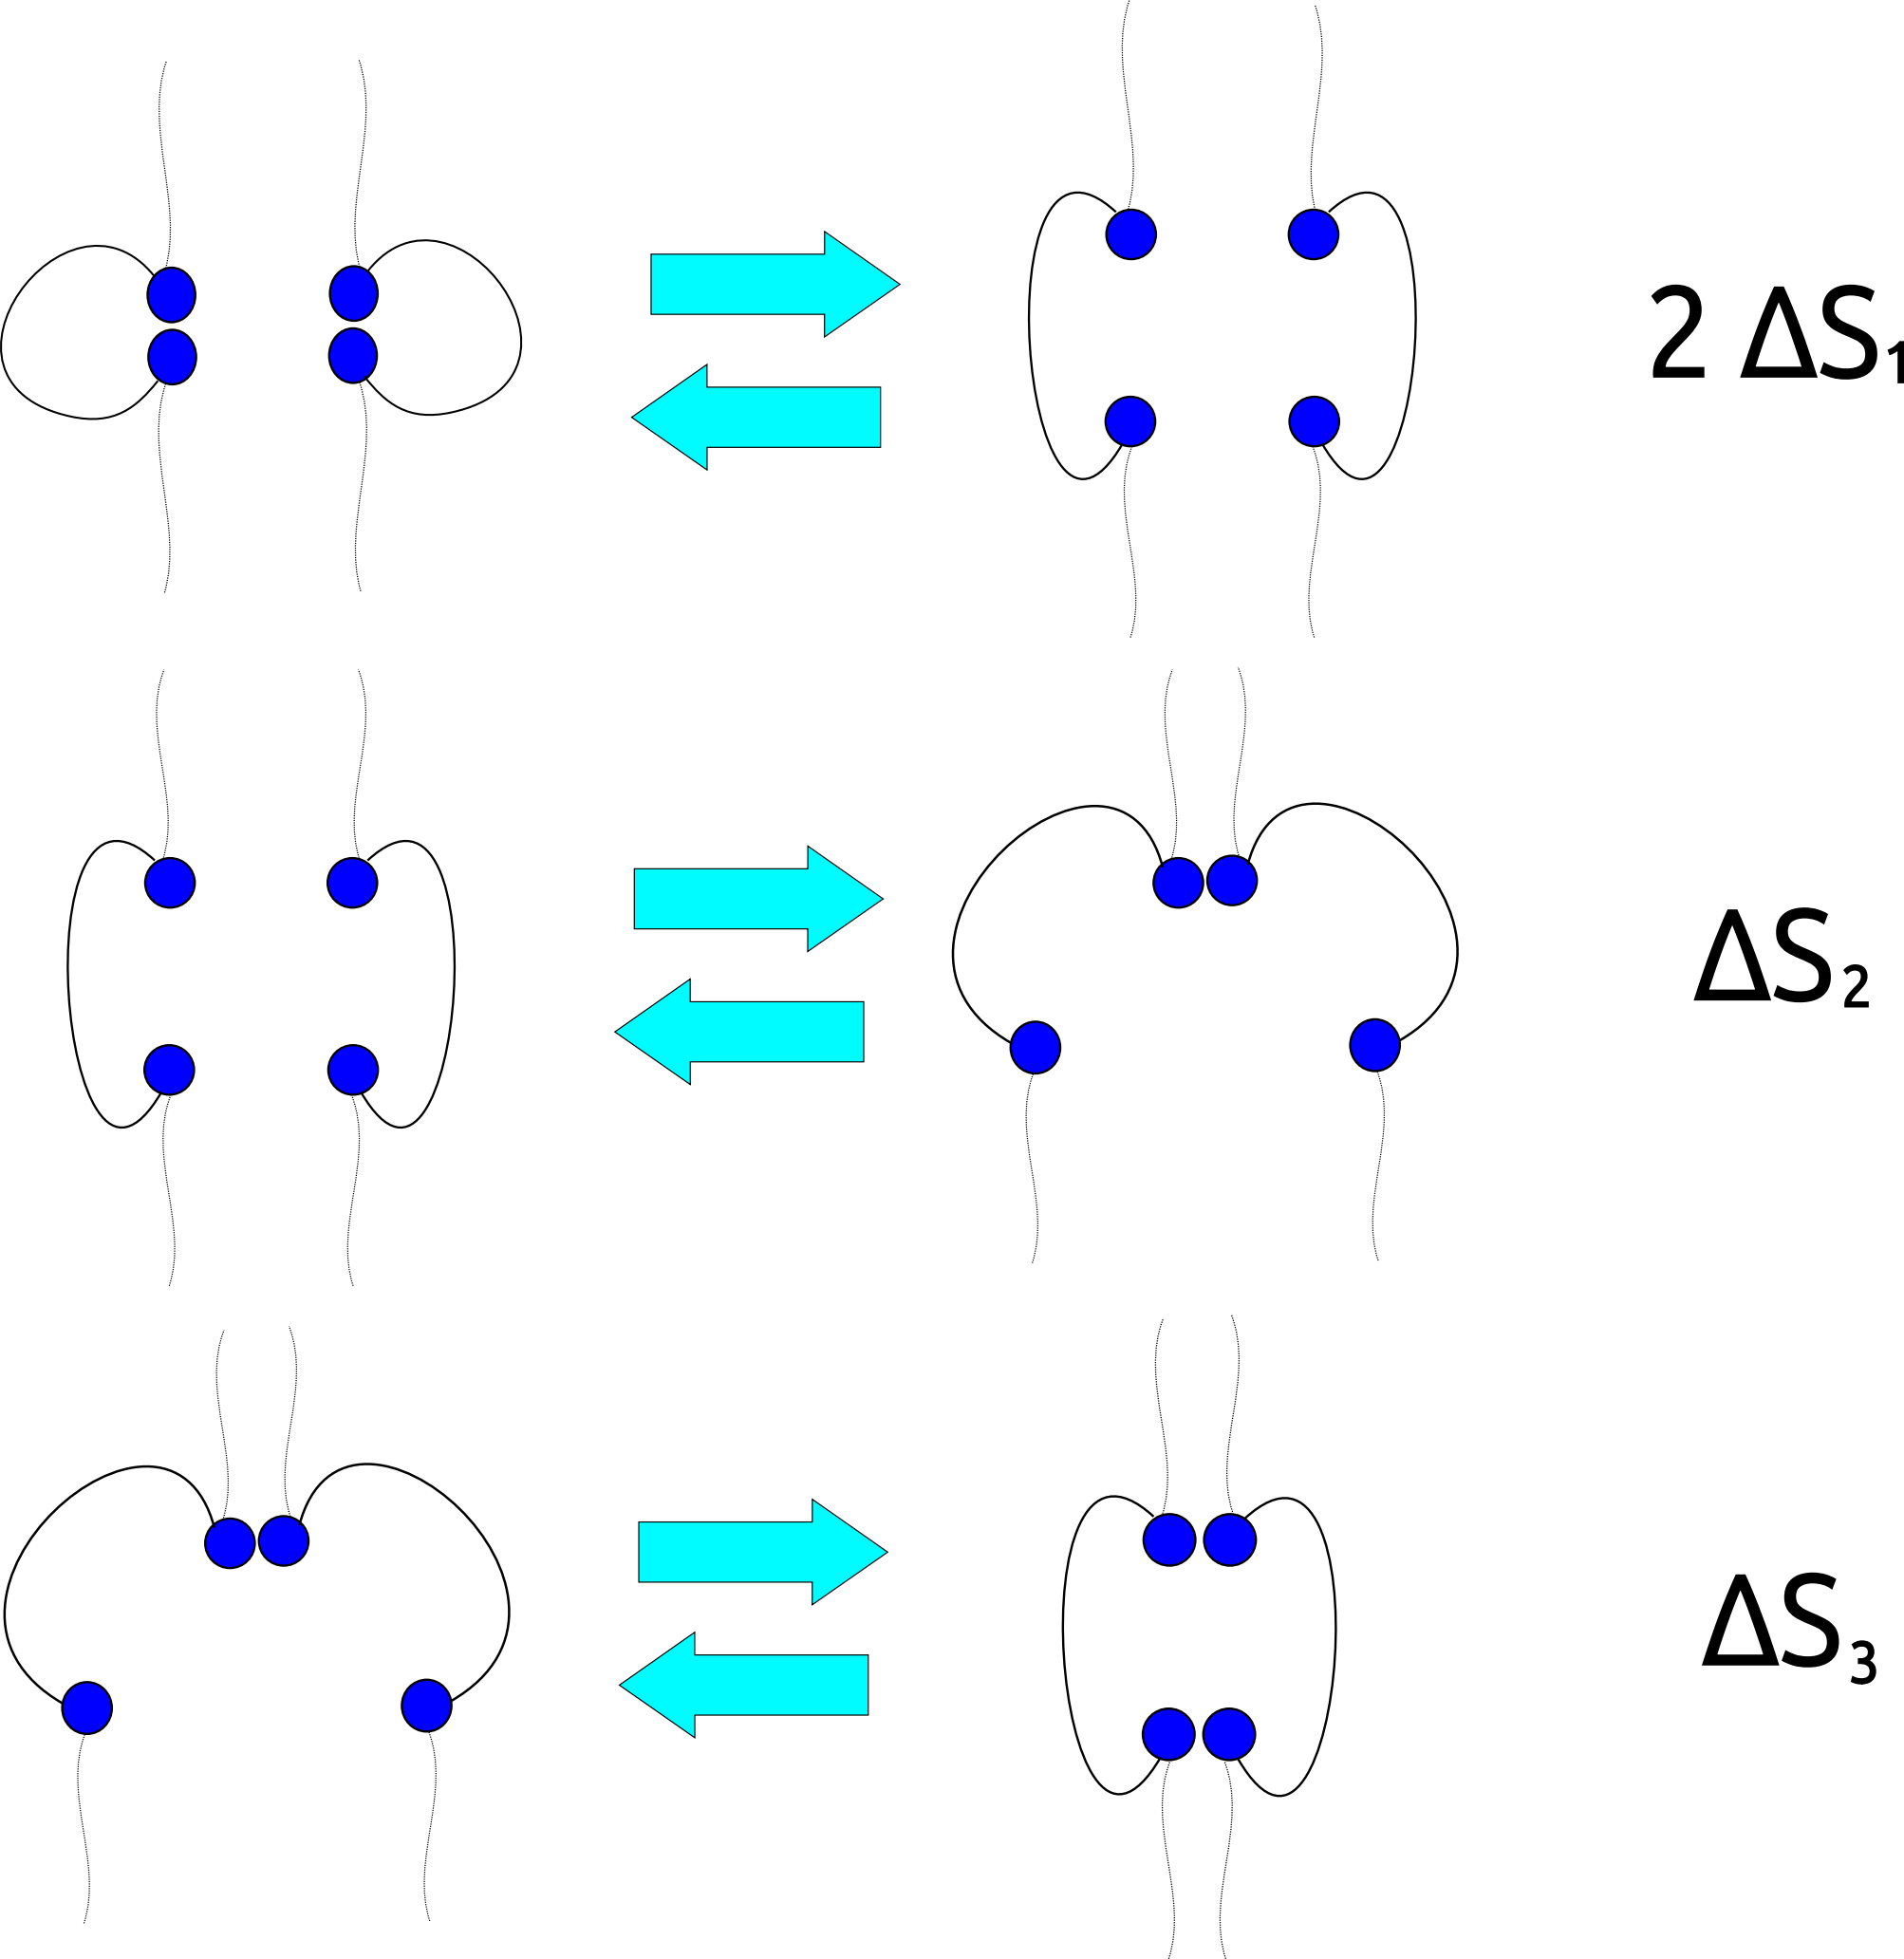

Supplement: Supplementary file 1 [file appendix.pdf]
